# Supplementary material for: Unsupervised Feature Clustering Improves Contrastive Representation Learning for Medical Image Segmentation
Source: arXiv:2211.08557 source file (2022-11-15)
Supplement: Supplementary file 1 [file section6_appendix.tex]

\subsection{Limitation of Global Contrastive with Domain Knowledge}
 
\setcounter{figure}{0}
\begin{figure}
    \centering
    \includegraphics[width=1\linewidth]{global_mmwhs.pdf}
    \caption{Example of three MMWHS MRI volumes' slices in four partitions.}
    \label{fig:global}
\end{figure}

To involve domain specific knowledge for image-wise representation learning, \cite{chaitanya2020contrastive} divided all medical volumes into four partitions and assumed that slices coming from the same partition contain similar structure information though belonging to different volumes.
From Fig.~\ref{fig:global}, we can see that the slices at partition 2 from those three volumes look similar and can be viewed as positive pair to each other. 
However, it is not the case for partition 1, 3, and 4, which is caused by the variation among different patients. 
On the other hand, the slices number for MMWHS is around 200~300, only four partitions result in that even for slices of the same partition of the same volume could look dissimilar.
Increasing the number of partition might increase the false negative cases, for example, the difference between the end of partition 1 and the first slice of partition 2 is actually minor.
